# Supplementary material for: Benchmarking EEG Foundation Models at Scale: Lessons from 20,000 Evaluations
Source: arXiv:2609.32743 source file (2026-09-26)
Supplement: Supplementary file 1 [file appendix_body_setup.tex]

\makeatletter
\@ifundefined{NC@find@L}{\newcolumntype{L}[1]{>{\raggedright\arraybackslash}p{#1}}}{}
\@ifundefined{NC@find@T}{\newcolumntype{T}[1]{>{\raggedright\arraybackslash}p{#1}}}{}
\@ifundefined{NC@find@C}{\newcolumntype{C}[1]{>{\centering\arraybackslash}p{#1}}}{}
\@ifundefined{appendix@LT@makecaption}{%
  \let\appendix@LT@makecaption\LT@makecaption
  \def\LT@makecaption#1#2#3{%
    \appendix@LT@makecaption{\small#1}{#2}{#3}%
  }%
  % TeX Live 2026's mark extraction trial-splits longtable page boxes.  The
  % package's \vss footer fillers contain infinite shrink and therefore emit a
  % harmless diagnostic on every longtable page.  Preserve the bottom fill but
  % bound its shrink component to 4pt, enough for small row-rounding excesses.
  \patchcmd{\LT@output}{\copy\LT@foot\vss}{\copy\LT@foot\vskip\z@\@plus1fil\@minus4pt\relax}{}{}
  \patchcmd{\LT@output}{\copy\LT@foot\vss}{\copy\LT@foot\vskip\z@\@plus1fil\@minus4pt\relax}{}{}
}{}
\makeatother

\providecolor{AppBaselineCell}{HTML}{F2F4F7}
\providecolor{AppFMCell}{HTML}{EAF4EF}
\providecolor{AppProtocolGainBlue}{HTML}{0F4D92}
\providecolor{AppProtocolLossRed}{HTML}{B5524A}
\providecommand{\BenchName}{EEG-Arena}

% Keep appendix figures close to the relevant text without crowding captions.
\setlength{\textfloatsep}{10pt plus 2pt minus 2pt}
\setlength{\floatsep}{8pt plus 2pt minus 2pt}
\setlength{\intextsep}{10pt plus 2pt minus 2pt}
\setlength{\abovecaptionskip}{5pt}
\setlength{\belowcaptionskip}{2pt}
\setlength{\LTcapwidth}{\textwidth}
\raggedbottom
\makeatletter
\setlength{\@fptop}{0pt}
\setlength{\@fpsep}{8pt plus 1pt minus 1pt}
\setlength{\@fpbot}{0pt plus 1fil}
\makeatother
\setcounter{topnumber}{3}
\setcounter{bottomnumber}{2}
\setcounter{totalnumber}{6}
\renewcommand{\topfraction}{0.95}
\renewcommand{\bottomfraction}{0.75}
\renewcommand{\textfraction}{0.03}
\renewcommand{\floatpagefraction}{0.65}
